# Supplementary material for: Defending Multimodal Fusion Models against Single-Source Adversaries
Source: arXiv:2206.12714 source file (2022-06-25)
Supplement: Supplementary file 12 [file results_dump.tex]

\begin{table*}[t]
\centering
\tiny
\begin{tabular}{|c|c|c|c|c|c|c|c|c|c|c|c|c|c|c|c|c|c|}
\hline
Model & \multicolumn{3}{c|}{Perturbed Vision} & Model & \multicolumn{3}{c|}{Perturbed Motion} & Model & \multicolumn{3}{c|}{Perturbed Audio} \\ \hline
 & Clean & Adv & Adv-F & & Clean & Adv & Adv-F & & Clean & Adv & Adv-F \\ \hline
Vision (LB) & 18.7 (54.2) & 0.0 (0.8) & 0.0 (0.0) &  Motion (LB) & 19.0 (48.4) & 0.0 (0.5) & 0.0 (0.0) &   Audio (LB) & 12.1 (35.9) & 0.0 (0.1) & 0.0 (0.0) \\ \hline
Concat Fusion & 30.2 (60.8) & 0.1 (8.9) & 0.0 (2.8) &   Concat Fusion & 30.2 (60.8) & 0.1 (7.5) & 0.0 (1.8) &   Concat Fusion & 30.2 (60.8) & 0.2 (8.1) & 0.0 (1.5) \\ \hline
Mean Fusion & 27.9 (59.7) & 0.0 (20.2) & 0.0 (8.8) &   Mean Fusion & 27.9 (59.7) & 0.0 (10.7) & 0.0 (10.7) &   Mean Fusion & 27.9 (59.7) & 0.0 (4.6) & 0.0 (4.6) \\ \hline
Motion+Audio (UB) & 21.9 (52.2) & 21.9 (52.2) & 21.9 (52.2) &   Vision+Audio (UB) & 23.8 (55.9) & 23.8 (55.9) & 23.8 (55.9) &   Motion+Audio (UB) & 25.6 (58.2) & 25.6 (58.2) & 25.6 (58.2) \\ \hline
\end{tabular}
\vspace{0.1cm}
\caption{Top-1 classification accuracy results on EPIC-Kitchens dataset. Higher is better. Standard multimodal fusion layers (mean, concat) are evaluated under single-source adversarial perturbations. LB = lower bound given by a unimodal model. UB = upper bound given by a multimodal model that excludes the perturbed modality.  Although there are three input modalities, perturbations (Adv, Adv-F) on a single modality are surprisingly effective, even when the adversary does not have access to the fusion layer weights (Adv-F). \karren{Full tables with results of top-5 classification accuracy, feature-level attack, noisy and mismatch corruptions are relegated to Supplementary Material but should be mentioned in the text.}}
\label{table:standard-fusion-epic-kitchens}
\end{table*}

\begin{table*}[t]
\centering
\tiny
\begin{tabular}{|c|c|c|c|c|c|c|c|c|c|c|c|c|c|c|c|c|c|}
\hline
Car detection & \multicolumn{3}{c|}{Perturbed RGB} & Model & \multicolumn{3}{c|}{Perturbed LIDAR} & Model & \multicolumn{3}{c|}{Perturbed Stereo} \\ \hline
 & Clean & Adv & Adv-F & & Clean & Adv & Adv-F & & Clean & Adv & Adv-F \\ \hline
RGB (LB) & 18.7 (54.2) & 0.0 (0.8) & 0.0 (0.0) &  %
LIDAR (LB) & 19.0 (48.4) & 0.0 (0.5) & 0.0 (0.0) & %
Stereo (LB) & 12.1 (35.9) & 0.0 (0.1) & 0.0 (0.0) \\ \hline
Concat Fusion & 30.2 (60.8) & 0.1 (8.9) & 0.0 (2.8) &  %
Concat Fusion & 30.2 (60.8) & 0.1 (7.5) & 0.0 (1.8) & %
Concat Fusion & 30.2 (60.8) & 0.2 (8.1) & 0.0 (1.5) \\ \hline
Mean Fusion & 27.9 (59.7) & 0.0 (20.2) & 0.0 (8.8) & %
Mean Fusion & 27.9 (59.7) & 0.0 (10.7) & 0.0 (10.7) &  %
Mean Fusion & 27.9 (59.7) & 0.0 (4.6) & 0.0 (4.6) \\ \hline
LIDAR+Stereo (UB) & 21.9 (52.2) & 21.9 (52.2) & 21.9 (52.2) & %
RGB+Stereo (UB) & 23.8 (55.9) & 23.8 (55.9) & 23.8 (55.9) &  %
RGB+LIDAR (UB) & 25.6 (58.2) & 25.6 (58.2) & 25.6 (58.2) \\ \hline \hline
Pedestrian detection & \multicolumn{3}{c|}{Perturbed RGB} & Model & \multicolumn{3}{c|}{Perturbed LIDAR} & Model & \multicolumn{3}{c|}{Perturbed Stereo} \\ \hline
 & Clean & Adv & Adv-F & & Clean & Adv & Adv-F & & Clean & Adv & Adv-F \\ \hline
RGB (LB) & 18.7 (54.2) & 0.0 (0.8) & 0.0 (0.0) &  %
LIDAR (LB) & 19.0 (48.4) & 0.0 (0.5) & 0.0 (0.0) & %
Stereo (LB) & 12.1 (35.9) & 0.0 (0.1) & 0.0 (0.0) \\ \hline
Concat Fusion & 30.2 (60.8) & 0.1 (8.9) & 0.0 (2.8) &  %
Concat Fusion & 30.2 (60.8) & 0.1 (7.5) & 0.0 (1.8) & %
Concat Fusion & 30.2 (60.8) & 0.2 (8.1) & 0.0 (1.5) \\ \hline
Mean Fusion & 27.9 (59.7) & 0.0 (20.2) & 0.0 (8.8) & %
Mean Fusion & 27.9 (59.7) & 0.0 (10.7) & 0.0 (10.7) &  %
Mean Fusion & 27.9 (59.7) & 0.0 (4.6) & 0.0 (4.6) \\ \hline
LIDAR+Stereo (UB) & 21.9 (52.2) & 21.9 (52.2) & 21.9 (52.2) & %
RGB+Stereo (UB) & 23.8 (55.9) & 23.8 (55.9) & 23.8 (55.9) &  %
RGB+LIDAR (UB) & 25.6 (58.2) & 25.6 (58.2) & 25.6 (58.2) \\ \hline \hline
Cyclist detection & \multicolumn{3}{c|}{Perturbed RGB} & Model & \multicolumn{3}{c|}{Perturbed LIDAR} & Model & \multicolumn{3}{c|}{Perturbed Stereo} \\ \hline
 & Clean & Adv & Adv-F & & Clean & Adv & Adv-F & & Clean & Adv & Adv-F \\ \hline
RGB (LB) & 18.7 (54.2) & 0.0 (0.8) & 0.0 (0.0) &  %
LIDAR (LB) & 19.0 (48.4) & 0.0 (0.5) & 0.0 (0.0) & %
Stereo (LB) & 12.1 (35.9) & 0.0 (0.1) & 0.0 (0.0) \\ \hline
Concat Fusion & 30.2 (60.8) & 0.1 (8.9) & 0.0 (2.8) &  %
Concat Fusion & 30.2 (60.8) & 0.1 (7.5) & 0.0 (1.8) & %
Concat Fusion & 30.2 (60.8) & 0.2 (8.1) & 0.0 (1.5) \\ \hline
Mean Fusion & 27.9 (59.7) & 0.0 (20.2) & 0.0 (8.8) & %
Mean Fusion & 27.9 (59.7) & 0.0 (10.7) & 0.0 (10.7) &  %
Mean Fusion & 27.9 (59.7) & 0.0 (4.6) & 0.0 (4.6) \\ \hline
LIDAR+Stereo (UB) & 21.9 (52.2) & 21.9 (52.2) & 21.9 (52.2) & %
RGB+Stereo (UB) & 23.8 (55.9) & 23.8 (55.9) & 23.8 (55.9) &  %
RGB+LIDAR (UB) & 25.6 (58.2) & 25.6 (58.2) & 25.6 (58.2) \\ \hline \hline

\end{tabular}
\vspace{0.1cm}
\caption{Average precision results on the EPIC-Kitchens dataset for car, pedestrian, and cyclist object classes. Higher is better. Standard multimodal fusion layers (mean, concat) are evaluated under single-source adversarial perturbations. Evaluation on Easy/Medium/Hard examples, following guidelines of KITTI evaluation server. LB = lower bound given by a unimodal model. UB = upper bound given by a multimodal model that excludes the perturbed modality. Although there are three input modalities, perturbations (Adv, Adv-F) on a single modality are surprisingly effective, even when the adversary does not have access to the fusion layer weights (Adv-F).}
\label{table:standard-fusion-kitti}
\end{table*}

\begin{table*}[]
\centering
\tiny
\begin{tabular}{|c|l|l|l|l|l|l|l|l|l|l|l|l|}
\hline
\textbf{Fusion} &
  \multicolumn{3}{c|}{Clean} &
  \multicolumn{3}{c|}{\begin{tabular}[c]{@{}c@{}}Visual \\ Perturbation\end{tabular}} &
  \multicolumn{3}{c|}{\begin{tabular}[c]{@{}c@{}}Motion \\ Perturbation\end{tabular}} &
  \multicolumn{3}{c|}{\begin{tabular}[c]{@{}c@{}}Audio \\ Perturbation\end{tabular}} \\ \hline
\textbf{} &
  \multicolumn{1}{c|}{\textbf{Verb}} &
  \multicolumn{1}{c|}{\textbf{Noun}} &
  \multicolumn{1}{c|}{\textbf{Action}} &
  \multicolumn{1}{c|}{\textbf{Verb}} &
  \multicolumn{1}{c|}{\textbf{Noun}} &
  \multicolumn{1}{c|}{\textbf{Action}} &
  \multicolumn{1}{c|}{\textbf{Verb}} &
  \multicolumn{1}{c|}{\textbf{Noun}} &
  \multicolumn{1}{c|}{\textbf{Action}} &
  \multicolumn{1}{c|}{\textbf{Verb}} &
  \multicolumn{1}{c|}{\textbf{Noun}} &
  \multicolumn{1}{c|}{\textbf{Action}} \\ \hline
\textbf{Concat Fusion} &
  59.0 (86.1) &
  42.1 (66.5) &
  30.2 (60.8) &
  0.1 (25.0) &
  0.0 (7.3) &
  0.0   (4.0) &
  0.2   (24.6) &
  0.0 (5.1) &
  0.0 (2.7) &
  0.1 (21.2) &
  0.0 (6.8) &
  0.0 (3.5) \\ \hline
\textbf{Mean Fusion} &
  56.8 (85.9) &
  40.4 (66.1) &
  27.6 (59.7) &
  0.3 (58.1) &
  0.8 (15.8) &
  0.0 (11.8) &
  0.3 (64.2) &
  0.3 (14.3) &
  0.0 (12.0) &
  0.4 (48.0) &
  0.3 (16.9) &
  0.0 (12.0) \\ \hhline{|=|=|=|=|=|=|=|=|=|=|=|=|=|}
\textbf{Concat Fusion} &
  61.2 (86.7) &
  \textbf{43.1 (68.9)} &
  30.5 (62.3) &
  22.3   (76.3) &
  11.6   (37.2) &
  6.6   (34.9) &
  25.4 (78.6) &
  24.6   (52.3) &
  12.0 (46.5) &
  20.4   (77.6) &
  17.7 (47.5) &
  8.0 (43.2) \\ \hline
\textbf{Feature Gating} &
  60.9 (87.6) &
  43.0 (68.7) &
  30.6 (62.8) &
  26.0 (77.9) &
  10.9 (42.0) &
  6.2 (39.0) &
  35.9 (83.6) &
  26.9 (58.3) &
  14.3 (52.5) &
  21.3 (79.9) &
  16.2 (51.4) &
  7.0 (47.2) \\ \hline
\textbf{Ours} &
  \textbf{61.5 (88.2)} &
  42.5 (68.4) &
  \textbf{31.4 (63.0)} &
  \textbf{48.0 (83.2)} &
  \textbf{24.2   (53.2)} &
  \textbf{16.8 (48.9)} &
  \textbf{48.5 (85.2)} &
  \textbf{35.6 (63.8)} &
  \textbf{22.1 (57.4)} &
  \textbf{46.5 (85.2)} &
  \textbf{33.3 (62.3)} &
  \textbf{22.1 (57.1)} \\ \hline
\end{tabular}
\vspace{0.1cm}
\caption{Top-1 (Top-5) classification accuracy results on EPIC-Kitchens dataset under clean data (columns 2-4) and single-source adversarial perturbations (columns 5-12) on each modality. Higher is better. \textbf{Note 1}: Adversarial training of all fusion layers (rows 5-7) improves robustness to single-source  without negatively impacting clean accuracy compared to clean training (rows 3-4); in fact, clean accuracy is slightly improved. \textbf{Note 2}: Our fusion layer (row 7) significantly improves single-source adversarial robustness over existing fusion layers (rows 5-6). }
\label{table:standard-fusion-kitti}
\end{table*}

\begin{table*}
\begin{center}
\begin{tabular}{|l|c|c|c|c|c|}
\hline
Model & Clean input & Audio attack & Video attack  & Text attack \\
\hline\hline
Naiive concat. fusion & 78.09 / 46.14& 53.21 / 20.51 & 43.15 / 18.17 & 33.14 / 8.23 \\
Naiive mean fusion & 81.82 / 46.69 & 56.92 / 21.38 & 51.23 / 19.75 & 39.50 / 9.97\\
Context-gated concat. fusion &78.82 / 46.37&69.31 / 38.26&64.23 / 31.88&59.39 / 25.14 \\
Context-gated mean fusion &82.03 / 46.89&73.18 / 40.06&69.94 / 38.20& 62.13 / 31.20\\
\hline
\end{tabular}
\end{center}
\caption{Binary / Seven-class classification results (\%) of naiive fusion models and the proposed context-gating under end-to-end white-box attack on MOSI}
\end{table*}

\begin{table*}[t]
\centering
\tiny
\begin{tabular}{|c|c|c|c|c|c|c|c|c|c|c|c|c|c|c|c|c|c|}
\hline
Model & \multicolumn{3}{c|}{Perturbed Vision} & Model & \multicolumn{3}{c|}{Perturbed Motion} & Model & \multicolumn{3}{c|}{Perturbed Audio} \\ \hline
 & Clean & Adv & Adv-F & & Clean & Adv & Adv-F & & Clean & Adv & Adv-F \\ \hline
Vision (LB) & 18.7 (54.2) & 0.0 (0.8) & 0.0 (0.0) &  Motion (LB) & 19.0 (48.4) & 0.0 (0.5) & 0.0 (0.0) &   Audio (LB) & 12.1 (35.9) & 0.0 (0.1) & 0.0 (0.0) \\ \hline
Concat Fusion & 30.2 (60.8) & 0.1 (8.9) & 0.0 (2.8) &   Concat Fusion & 30.2 (60.8) & 0.1 (7.5) & 0.0 (1.8) &   Concat Fusion & 30.2 (60.8) & 0.2 (8.1) & 0.0 (1.5) \\ \hline
Mean Fusion & 27.9 (59.7) & 0.0 (20.2) & 0.0 (8.8) &   Mean Fusion & 27.9 (59.7) & 0.0 (10.7) & 0.0 (10.7) &   Mean Fusion & 27.9 (59.7) & 0.0 (4.6) & 0.0 (4.6) \\ \hline
Motion+Audio (UB) & 21.9 (52.2) & 21.9 (52.2) & 21.9 (52.2) &   Vision+Audio (UB) & 23.8 (55.9) & 23.8 (55.9) & 23.8 (55.9) &   Motion+Audio (UB) & 25.6 (58.2) & 25.6 (58.2) & 25.6 (58.2) \\ \hline
\end{tabular}
\vspace{0.1cm}
\caption{Top-1 classification accuracy results on EPIC-Kitchens dataset. Higher is better. Standard multimodal fusion layers (mean, concat) are evaluated under single-source adversarial perturbations. LB = lower bound given by a unimodal model. UB = upper bound given by a multimodal model that excludes the perturbed modality.  Although there are three input modalities, perturbations (Adv, Adv-F) on a single modality are surprisingly effective, even when the adversary does not have access to the fusion layer weights (Adv-F). \karren{Full tables with results of top-5 classification accuracy, feature-level attack, noisy and mismatch corruptions are relegated to Supplementary Material but should be mentioned in the text.}}
\label{table:standard-fusion-epic-kitchens}
\end{table*}

\begin{table*}[t]
\centering
\scriptsize
\begin{tabular}{|l|c|c|l|c|c|l|}
\hline
\textbf{Fusion} &
  \multicolumn{3}{c|}{\textbf{Clean}} &
  \multicolumn{3}{c|}{\textbf{\begin{tabular}[c]{@{}c@{}}Visual (RGB)\\ Perturbation\end{tabular}}} \\ \hline
\textbf{} &
  \textbf{Car} &
  \textbf{Ped} &
  \multicolumn{1}{c|}{\textbf{Cyc}} &
  \textbf{Car} &
  \textbf{Ped} &
  \multicolumn{1}{c|}{\textbf{Cyc}} \\ \hline
\textbf{Baseline} &
  96.1 / 93.5 / 86.8 &
  85.7 / 81.5 / 77.0 &
  93.2 / 87.7 / 83.2 &
  15.6 / 14.3 / 14.8 &
  13.6 / 10.7 / 10.3 &
  13.8 / 12.3 / 12.9 \\ \hline
\textbf{Mean} &
  96.5 / 93.6 / 86.6 &
  84.3 / 77.7 / 73.4 &
  91.9 / 86.7 / 81.8 &
  13.2 / 12.6 / 13.1 &
  18.1 / 15.2 / 14.2 &
  11.9 / 10.5 / 10.2 \\ \hline
\textbf{Concat} &
  \multicolumn{1}{l|}{80.5 / 71.4 / 67.3} &
  \multicolumn{1}{l|}{69.0 / 64.2 / 61.3} &
  75.7 / 80.0 / 75.3 &
  \multicolumn{1}{l|}{3.71 / 3.95 / 4.62} &
  \multicolumn{1}{l|}{16.9 / 15.4 / 14.3} &
  16.4 / 13.9 / 13.2 \\ \hline
\textbf{Feature-Gated} &
  \multicolumn{1}{l|}{90.6 / 89.4 / 82.8} &
  \multicolumn{1}{l|}{81.5 / 74.7 / 72.6} &
  92.9 / 84.6 / 81.8 &
  \multicolumn{1}{l|}{67.3 / 57.2 / 53.1} &
  \multicolumn{1}{l|}{62.0 / 54.2 / 50.7} &
  68.6 / 56.0 / 53.1 \\ \hline
\textbf{Ours} &
  \multicolumn{1}{l|}{95.6 / 90.6 / 83.9} &
  \multicolumn{1}{l|}{84.5 / 79.9 / 75.7} &
  90.4 / 85.4 / 80.6 &
  \multicolumn{1}{l|}{\textbf{89.6 / 85.1 / 78.9}} &
  \multicolumn{1}{l|}{\textbf{80.5 / 73.9 / 69.8}} &
  \textbf{87.9 / 82.3 / 77.6} \\ \hline
\textbf{$\Delta$} &
   &
   &
   &
   &
   &
   \\ \hline
\end{tabular}
\caption{Average Precision results for KITTI}
\label{table:kitti-robustness-results-1}
\end{table*}

\begin{table*}[t]
\centering
\scriptsize
\begin{tabular}{|l|c|c|l|c|c|l|}
\hline
\textbf{Fusion} &
  \multicolumn{3}{c|}{\textbf{\begin{tabular}[c]{@{}c@{}}Depth (Velo)\\ Perturbation\end{tabular}}} &
  \multicolumn{3}{c|}{\textbf{\begin{tabular}[c]{@{}c@{}}Stereo Disparity\\ Perturbation\end{tabular}}} \\ \hline
\textbf{} &
  \textbf{Car} &
  \textbf{Ped} &
  \multicolumn{1}{c|}{\textbf{Cyc}} &
  \textbf{Car} &
  \textbf{Ped} &
  \multicolumn{1}{c|}{\textbf{Cyc}} \\ \hline
\textbf{Baseline} &
  3.43 / 1.58 / 1.59 &
  11.3 / 11.1 / 11.4 &
  8.72 / 8.82 / 8.22 &
  7.37 / 3.57 / 3.44 &
  8.08 / 4.64 / 4.36 &
  9.13 / 7.23 / 7.72 \\ \hline
\textbf{Mean} &
  6.77 / 3.16 / 2.90 &
  13.7 / 12.9 / 12.8 &
  10.1 / 7.88 / 8.07 &
  6.88 / 3.08 / 2.73 &
  9.17 / 8.03 / 8.81 &
  12.2 / 7.77 / 7.28 \\ \hline
\textbf{Concat} &
  \multicolumn{1}{l|}{7.30 / 6.83 / 6.73} &
  \multicolumn{1}{l|}{24.4 / 20.6 / 18.9} &
  28.8 / 24.8 / 24.7 &
  \multicolumn{1}{l|}{10.1 / 9.39 / 9.50} &
  \multicolumn{1}{l|}{26.0 / 24.2 / 21.8} &
  25.7 / 24.7 / 23.8 \\ \hline
\textbf{Feature-Gated} &
  \multicolumn{1}{l|}{51.7 / 46.5 / 43.2} &
  \multicolumn{1}{l|}{53.5 / 45.7 / 42.1} &
  58.8 / 45.6 / 53.8 &
  \multicolumn{1}{l|}{43.9 / 41.6 / 38.8} &
  \multicolumn{1}{l|}{53.9 / 47.4 / 44.1} &
  60.0 / 48.8 / 46.8 \\ \hline
\textbf{Ours} &
  \multicolumn{1}{l|}{\textbf{92.8 / 87.8 / 79.4}} &
  \multicolumn{1}{l|}{\textbf{78.3 / 71.1 / 67.1}} &
  \textbf{88.9 / 85.8 / 81.1} &
  \multicolumn{1}{l|}{\textbf{92.8 / 89.8 / 83.1}} &
  \multicolumn{1}{l|}{\textbf{83.6 / 76.8 / 72.4}} &
  \textbf{88.1 / 84.7 / 79.9} \\ \hline
\textbf{$\Delta$} &
   &
   &
   &
   &
   &
   \\ \hline
\end{tabular}
\caption{Average Precision results for KITTI}
\label{table:kitti-robustness-results-2}
\end{table*}

\begin{table}[]
\begin{tabular}{|l|c|c|c|c|c|c|c|c|c|c|c|c|c|c|c|c|}
\hline
\multicolumn{17}{|c|}{\textbf{EPIC-Kitchens}} \\ \hline
\textbf{Odd-one-out network} &
  \multicolumn{4}{c|}{\textbf{Clean}} &
  \multicolumn{4}{c|}{\textbf{\begin{tabular}[c]{@{}c@{}}Visual\\ Perturbation\end{tabular}}} &
  \multicolumn{4}{c|}{\textbf{\begin{tabular}[c]{@{}c@{}}Motion\\ Perturbation\end{tabular}}} &
  \multicolumn{4}{c|}{\textbf{\begin{tabular}[c]{@{}c@{}}Audio\\ Perturbation\end{tabular}}} \\ \hline
\textbf{} &
  \textbf{Detect} &
  \textbf{Verb} &
  \textbf{Noun} &
  \textbf{Action} &
  \textbf{Detect} &
  \textbf{Verb} &
  \textbf{Noun} &
  \textbf{Action} &
  \textbf{Detect} &
  \textbf{Verb} &
  \textbf{Noun} &
  \textbf{Action} &
  \textbf{Detect} &
  \textbf{Verb} &
  \textbf{Noun} &
  \textbf{Action} \\ \hline
\textbf{Random} &
  25.0 &
  - &
  - &
  - &
  25.0 &
  - &
  - &
  - &
  25.0 &
  - &
  - &
  - &
  25.0 &
  - &
  - &
  - \\ \hline
\textbf{Unaligned features} &
  \textbf{66.8} &
  \textbf{61.5} &
  \textbf{42.5} &
  \textbf{31.4} &
  \textbf{73.4} &
  \textbf{48.0} &
  \textbf{24.2} &
  \textbf{16.8} &
  \textbf{88.6} &
  \textbf{48.5} &
  \textbf{35.6} &
  \textbf{21.1} &
  \textbf{84.7} &
  \textbf{46.5} &
  \textbf{33.3} &
  \textbf{22.1} \\ \hline
\textbf{\begin{tabular}[c]{@{}l@{}}Aligned features\\ (Logits)\end{tabular}} &
  55.9 &
  \textbf{61.5} &
  38.0 &
  31.2 &
  54.7 &
  38.7 &
  19.5 &
  13.1 &
  41.3 &
  37.0 &
  29.1 &
  16.7 &
  52.8 &
  31.1 &
  23.9 &
  13.8 \\ \hline
\multicolumn{17}{|c|}{\textbf{KITTI}} \\ \hline
\textbf{Odd-one-out network} &
  \multicolumn{4}{c|}{\textbf{Clean}} &
  \multicolumn{4}{c|}{\textbf{\begin{tabular}[c]{@{}c@{}}Visual (RGB)\\ Perturbation\end{tabular}}} &
  \multicolumn{4}{c|}{\textbf{\begin{tabular}[c]{@{}c@{}}Depth (Velo)\\ Perturbation\end{tabular}}} &
  \multicolumn{4}{c|}{\textbf{\begin{tabular}[c]{@{}c@{}}Stereo Disparity\\ Perturbation\end{tabular}}} \\ \hline
\textbf{} &
  \textbf{Detect} &
  \textbf{Car} &
  \textbf{Pedest.} &
  \textbf{Cyclist} &
  \textbf{Detect} &
  \textbf{Car} &
  \textbf{Pedest.} &
  \textbf{Cyclist} &
  \textbf{Detect} &
  \textbf{Car} &
  \textbf{Pedest.} &
  \textbf{Cyclist} &
  \textbf{Detect} &
  \textbf{Car} &
  \textbf{Pedest.} &
  \textbf{Cyclist} \\ \hline
\textbf{Random} &
  25.0 &
  - &
  - &
  - &
  25.0 &
  - &
  - &
  - &
  25.0 &
  - &
  - &
  - &
  25.0 &
  - &
  - &
  - \\ \hline
\textbf{Unaligned features} &
  \textbf{96.2} &
  \textbf{90.6} &
  \textbf{79.9} &
  \textbf{85.4} &
  \textbf{93.5} &
  \textbf{85.1} &
  \textbf{73.9} &
  \textbf{82.3} &
  \textbf{98.2} &
  \textbf{87.8} &
  \textbf{71.1} &
  \textbf{85.8} &
  \textbf{98.0} &
  \textbf{89.8} &
  \textbf{76.8} &
  \textbf{84.7} \\ \hline
\textbf{\begin{tabular}[c]{@{}l@{}}Aligned features\\ (Bounding Boxes)\end{tabular}} &
  91.9 &
  90.2 &
  76.1 &
  83.3 &
  86.8 &
  77.6 &
  66.5 &
  73.8 &
  94.4 &
  83.1 &
  64.8 &
  68.3 &
  90.4 &
  80.0 &
  65.1 &
  44.9 \\ \hline
\end{tabular}
\caption{Aligned v. unaligned features}
\end{table}
